# Supplementary material for: KITRO: Refining Human Mesh by 2D Clues and Kinematic-tree Rotation
Source: arXiv:2405.19833 source file (2024-05-30)
Supplement: Supplementary file 1 [file x_suppl_bkup.tex]

\clearpage
\setcounter{page}{1}
\maketitlesupplementary

% Reset the section counter
\setcounter{section}{0}
% Redefine the section numbering to use letters

\section{Details on Swing-Twist Decomposition} \label{supp:swingtwist}

\section{Proof-of-concept for Solution Selection} \label{supp:proofofconcept}

\section{Correctness Proof for \cref{eq:thetaupdating}} \label{supp:proof}

\section{More Ablation Studies} \label{supp:moreablation}

\section{Visulization of Samples Improvement Distribution} \label{supp:Distribution}

\section{Names of Joints and Bones on Kinematic-tree} \label{supp:nameKT}

\section{More Implementation Details}
Kinematic Tree. List all the bone that we are using.

Evaluation Metric: all neutral gender; include hard samples; average of 2 hips as base joint

\todo{alignment of 2dkp; }

Since we use Adam optimizer optimizer, we also perform ablation study on how

\todo{2d repro error; (rewind)}

\section{fully experiments}

\begin{table*}[t!]
    \centering
    \caption{Camera}
    \begin{tabular}{lccccccc}
        \hline 
        & \multicolumn{3}{c}{3DPW} & & \multicolumn{3}{c}{Human3.6M} \\
        \cline { 2 - 4 } \cline { 6 - 8 }
        Method & PA-MPJPE $\downarrow$ & MPJPE $\downarrow$ & PVE $\downarrow$ & & PA-MPJPE $\downarrow$ & MPJPE $\downarrow$ & PVE $\downarrow$ \\
        \hline 
        KAR w/o CE & 28.53 & 46.68 & 57.76     & & 21.30 & \textbf{33.22} & \textbf{41.12}\\
        KAR w/o Eq.\ref{eq:cammovingavg} & 27.99 & 50.21 & 61.11     & & 21.21 & 37.49 & 46.59\\
        \hline
        KAR  & \textbf{27.67} & \textbf{43.53} & \textbf{53.44}      & & \textbf{21.04} & 34.50 & 42.88\\
        \hline
    \end{tabular}
    \label{tab:allcam}
\end{table*}

\begin{table*}[t!]
    \centering
    \caption{Shape}
    \begin{tabular}{lccccccc}
        \hline 
        & \multicolumn{3}{c}{3DPW} & & \multicolumn{3}{c}{Human3.6M} \\
        \cline { 2 - 4 } \cline { 6 - 8 }
        Method & PA-MPJPE $\downarrow$ & MPJPE $\downarrow$ & PVE $\downarrow$ & & PA-MPJPE $\downarrow$ & MPJPE $\downarrow$ & PVE $\downarrow$ \\
        \hline 
        KAR w/o SO & 35.00 & 69.02 & 84.25     & & 35.40 & 55.01 & 66.18\\
        2D reproj. loss & 32.60 & 52.60 & 64.45     & & 30.38 & 50.32 & 62.41\\
        \hline
        KAR  & \textbf{27.67} & \textbf{43.53} & \textbf{53.44}      & & \textbf{21.04} & \textbf{34.50} & \textbf{42.88}\\
        \hline
    \end{tabular}
    \label{tab:allshape}
\end{table*}

\begin{table*}[t!]
    \centering
    \caption{Shape iteration number}
    \begin{tabular}{lccccccc}
        \hline 
        & \multicolumn{3}{c}{3DPW} & & \multicolumn{3}{c}{Human3.6M} \\
        \cline { 2 - 4 } \cline { 6 - 8 }
        Method & PA-MPJPE $\downarrow$ & MPJPE $\downarrow$ & PVE $\downarrow$ & & PA-MPJPE $\downarrow$ & MPJPE $\downarrow$ & PVE $\downarrow$ \\
        \hline 
        iter 100  & 31.30 & 46.84 & 58.78     & &  &  & \\
        iter 50  & 29.36 & 44.12 & 54.68     & &  &  & \\
        iter 40  & 28.79 & 43.34 & 53.51     & &  &  & \\
        iter 30  & 28.15 & 42.34 & 52.09     & &  &  & \\
        iter 20  & 27.56 & 42.07 & 51.55     & &  &  & \\
        iter 10  & 27.67 & 43.53 & 53.44     & &  &  & \\
        iter 5 & 28.57 & 47.31 & 58.74     & &  &  & \\
        iter 1 & 34.91 & 69.24 & 81.99     & &  &  & \\
        iter 0 & 43.76 & 73.67 & 91.58     & &  &  & \\
        \hline
        KAR (iter 10)  & \textbf{27.67} & \textbf{43.53} & \textbf{53.44}      & & \textbf{21.04} & \textbf{34.50} & \textbf{42.88}\\
        \hline
    \end{tabular}
    \label{tab:shapeiter}
\end{table*}

\begin{table*}[t!]
    \centering
    \caption{Shape learning rate}
    \begin{tabular}{lccccccc}
        \hline 
        & \multicolumn{3}{c}{3DPW} & & \multicolumn{3}{c}{Human3.6M} \\
        \cline { 2 - 4 } \cline { 6 - 8 }
        Method & PA-MPJPE $\downarrow$ & MPJPE $\downarrow$ & PVE $\downarrow$ & & PA-MPJPE $\downarrow$ & MPJPE $\downarrow$ & PVE $\downarrow$ \\
        \hline 
        lr 1.0  & 38.29 & 61.78 & 76.17     & &  &  & \\
        lr 0.5  & 31.68 & 49.26 & 60.33     & &  &  & \\
        lr 0.2  & 28.23 & 43.47 & 53.00     & &  &  & \\
        lr 0.1  & 27.67 & 43.53 & 53.44     & &  &  & \\
        lr 0.05  & 28.25 & 47.78 & 58.90     & &  &  & \\
        lr 0.01 & 32.71 & 63.59 & 76.75     & &  &  & \\
        \hline
        KAR (lr 0.1)  & \textbf{27.67} & \textbf{43.53} & \textbf{53.44}      & & \textbf{21.04} & \textbf{34.50} & \textbf{42.88}\\
        \hline
    \end{tabular}
    \label{tab:shapeiter}
\end{table*}

\begin{table*}[t!]
    \centering
    \caption{Pose}
    \begin{tabular}{lccccccc}
        \hline 
        & \multicolumn{3}{c}{3DPW} & & \multicolumn{3}{c}{Human3.6M} \\
        \cline { 2 - 4 } \cline { 6 - 8 }
        Method & PA-MPJPE $\downarrow$ & MPJPE $\downarrow$ & PVE $\downarrow$ & & PA-MPJPE $\downarrow$ & MPJPE $\downarrow$ & PVE $\downarrow$ \\
        \hline 
        KAR w/o PR & 44.57 & 80.03 & 95.71     & & 37.98 & 65.54 & 83.60\\
        KAR w/o DecisionTree & 28.78 & 44.52 & 54.43     & & 21.61 & 34.93 & 43.34\\
        KAR w/o rewind & 28.10 & 44.39 & 54.27     & & 21.46 & 35.06 & 43.37\\
        KAR w/o reweighting & 32.18 & 52.15 & 63.82     & & 24.10 & 40.23 & 48.45\\
        \hline
        KAR  & \textbf{27.67} & \textbf{43.53} & \textbf{53.44}      & & \textbf{21.04} & \textbf{34.50} & \textbf{42.88}\\
        \hline
    \end{tabular}
    \label{tab:allpose}
\end{table*}

\begin{table*}[t!]
    \centering
    \caption{Loop number}
    \begin{tabular}{lccccccc}
        \hline 
        & \multicolumn{3}{c}{3DPW} & & \multicolumn{3}{c}{Human3.6M} \\
        \cline { 2 - 4 } \cline { 6 - 8 }
        Method & PA-MPJPE $\downarrow$ & MPJPE $\downarrow$ & PVE $\downarrow$ & & PA-MPJPE $\downarrow$ & MPJPE $\downarrow$ & PVE $\downarrow$ \\
        \hline 
        loop 50  & 29.08 & 45.89 & 56.53     & &  &  & \\
        loop 20  & 27.83 & 43.35 & 53.37     & &  &  & \\
        loop 5  & 27.76 & 44.05 & 54.09     & &  &  & \\
        loop 1 & 33.05 & 53.37 & 66.36     & &  &  & \\
        loop 0 (baseline) & 43.0 & 69.0 & 81.2     & & 36.16 & 55.18 & 74.46\\
        \hline
        KAR (loop 10)  & \textbf{27.67} & \textbf{43.53} & \textbf{53.44}      & & \textbf{21.04} & \textbf{34.50} & \textbf{42.88}\\
        \hline
    \end{tabular}
    \label{tab:loopnum}
\end{table*}

\begin{table*}[t!]
    \centering
    \caption{SOTA comparision on 3DPW and HM36. (*) denotes the result of ours reproduction.}
    \begin{tabular}{lccccccc}
        \hline 
        & \multicolumn{3}{c}{3DPW} & & \multicolumn{3}{c}{Human3.6M} \\
        \cline { 2 - 4 } \cline { 6 - 8 }
        Method & PA-MPJPE $\downarrow$ & MPJPE $\downarrow$ & PVE $\downarrow$ & & PA-MPJPE $\downarrow$ & MPJPE $\downarrow$ & PVE $\downarrow$ \\
        \hline 
        Baseline (report) & 43.0 & 69.0 & 81.2     & & - & - & - \\
        Baseline (w/o GT2D) & 43.76 & 73.67 & 91.58     & & 36.16 & 55.18 & 74.46 \\
        \hline 
        DynaBOA & 40.4 & 65.5 & 82.0    & & - & - & -\\
        Pose2Mesh & 34.6 & 65.1 & -     & & 35.3 & 51.1 & -\\
        CLIFF (w/ GT2D) diff.criterion  & 32.8 & 52.8 & 61.5      & & - & - & -\\
        CLIFF* (w/ GT2D 3DPW) & 32.04 & 55.83 & 71.95      & & 36.16 & 55.18 & 74.46\\
        CLIFF* (w/ GT2D HM36) & 46.17 & 77.85 & 94.71      & & 25.88 & 42.79 & 60.60\\
        CLIFF+SMPLify* & 32.63 & 58.89 & 75.90      & & 28.71 & 45.62 & 63.77\\
        \hline
        KAR \textbf{(Ours)}  & \textbf{27.67} & \textbf{43.53} & \textbf{53.44}      & & \textbf{21.04} & \textbf{34.50} & \textbf{42.88}\\
        \hline
        KAR (Ours on CLIFF 3DPW)  & 26.21 & 46.96 & 57.53      & & 25.14 & 41.75 & 51.67\\
        KAR (Ours on CLIFF HM36)  & 28.22 & 44.35 & 54.38      & & 20.28 & 34.77 & 43.37\\
        \hline
        SPIN-baseline  & 59.97 & 102.12 & 130.62      & & 40.57 & 61.65 & 83.61\\
        SPIN\textbf{+ours}  & 42.46 & 67.12 & 80.25      & & 26.45 & 37.91 & 47.46\\
        SPIN+SMPLify* & 43.64(47.99) & 79.56(87.06) & 101.50(102.28)      & &  &  & \\
        \hline
        EFT-baseline  & 54.71 & 94.02 & 116.23      & & 44.54 & 68.00 & 89.43\\
        EFT\textbf{+ours}  & 32.34 & 49.14 & 59.28      & & 26.24 & 41.17 & 49.68 \\
        \hline
    \end{tabular}
    \label{tab:SOTA}
\end{table*}

\begin{table*}[t!]
    \centering
    \caption{Upper-bound study}
    \begin{tabular}{lccccccc}
        \hline 
        & \multicolumn{3}{c}{3DPW} & & \multicolumn{3}{c}{Human3.6M} \\
        \cline { 2 - 4 } \cline { 6 - 8 }
        Method & PA-MPJPE $\downarrow$ & MPJPE $\downarrow$ & PVE $\downarrow$ & & PA-MPJPE $\downarrow$ & MPJPE $\downarrow$ & PVE $\downarrow$ \\
        \hline 
        % GT intrinsic  & 29.08 & 45.89 & 56.53     & &  &  & \\
        GT camera translation  &  &  &      & &  &  & \\
        \hline
        GT shape  &  &  &      & &  &  & \\
        \hline
        GT hypothesis &  &  &      & &  &  & \\
        \hline
        KAR (loop 10)  & \textbf{27.67} & \textbf{43.53} & \textbf{53.44}      & & \textbf{21.04} & \textbf{34.50} & \textbf{42.88}\\
        \hline
    \end{tabular}
    \label{tab:loopnum}
\end{table*}

\begin{table*}[t!]
    \centering
    \caption{Upper-bound study}
    \begin{tabular}{cccccccccc}
        \hline 
        &&& \multicolumn{3}{c}{3DPW} & & \multicolumn{3}{c}{Human3.6M} \\
        \cline { 4 - 6 } \cline { 8 -  10}
        Camera & Shape & Pose & PA-MPJPE $\downarrow$ & MPJPE $\downarrow$ & PVE $\downarrow$ & & PA-MPJPE $\downarrow$ & MPJPE $\downarrow$ & PVE $\downarrow$ \\
        \hline 
        \ding{55} & \ding{55} & \ding{55} & 43.76 & 73.67 & 91.58     & & 36.16 & 55.18 & 74.46 \\
        \checkmark  & \ding{55} & \ding{55} & 43.76 & 73.67 & 91.58     & & 36.16 & 55.18 & 74.46\\
        \ding{55} & \checkmark & \ding{55}  & 44.31 & 69.92 & 83.26     & & 37.74 & 54.02 & 67.94\\        
        \ding{55} & \ding{55} &  \checkmark & 45.92 & 87.33 & 100.73     & & 34.87 & 52.63 & 68.09\\
        \checkmark & \checkmark  & \ding{55} & 44.57 & 80.03 & 95.71     & & 37.98 & 65.54 & 83.60\\
        \checkmark & \ding{55} & \checkmark & 35.00 & 69.02 & 84.25     & & 35.40 & 55.01 & 66.18\\
        \ding{55} & \checkmark & \checkmark  & 28.53 & 46.68 & 57.76     & & 21.30 & 33.22 & 41.12\\
        \checkmark & \checkmark & \checkmark & \textbf{27.67} & \textbf{43.53} & \textbf{53.44}      & & \textbf{21.04} & \textbf{34.50} & \textbf{42.88}\\
        \hline
    \end{tabular}
    \label{tab:allpose}
\end{table*}

% \section{Rationale}
% \label{sec:rationale}
% % 
% Having the supplementary compiled together with the main paper means that:
% % 
% \begin{itemize}
% \item The supplementary can back-reference sections of the main paper, for example, we can refer to \cref{sec:intro};
% \item The main paper can forward reference sub-sections within the supplementary explicitly (e.g. referring to a particular experiment); 
% \item When submitted to arXiv, the supplementary will already included at the end of the paper.
% \end{itemize}
% % 
% To split the supplementary pages from the main paper, you can use \href{https://support.apple.com/en-ca/guide/preview/prvw11793/mac#:~:text=Delete%20a%20page%20from%20a,or%20choose%20Edit%20%3E%20Delete).}{Preview (on macOS)}, \href{https://www.adobe.com/acrobat/how-to/delete-pages-from-pdf.html#:~:text=Choose%20%E2%80%9CTools%E2%80%9D%20%3E%20%E2%80%9COrganize,or%20pages%20from%20the%20file.}{Adobe Acrobat} (on all OSs), as well as \href{https://superuser.com/questions/517986/is-it-possible-to-delete-some-pages-of-a-pdf-document}{command line tools}.
